# Supplementary material for: Grounding Partially-Defined Events in Multimodal Data
Source: arXiv:2410.05267 source file (2024-10-07)
Supplement: Supplementary file 1 [file a02_data_analysis.tex]

\section{Supplementary \dsetname { }data analysis}
\label{appendix:data-analysis}
\subsection{Descriptions}
\subsection{Entity labels}
\subsection{Video length}
\subsection{Event list}
\subsection{Language distribution}
