# Supplementary material for: Grounding Partially-Defined Events in Multimodal Data
Source: arXiv:2410.05267 source file (2024-10-07)
Supplement: Supplementary file 2 [file a05_ablation_experiments.tex]

\section{Additional experiments}
\label{appendix:experiments}
