# Supplementary material for: Grounding Partially-Defined Events in Multimodal Data
Source: arXiv:2410.05267 source file (2024-10-07)
Supplement: Supplementary file 4 [file a09_vlm_info.tex]

\section{TimeChat Modeling Information}
\label{appendix:model-details}
