# Supplementary material for: Grounding Partially-Defined Events in Multimodal Data
Source: arXiv:2410.05267 source file (2024-10-07)
Supplement: Supplementary file 5 [file a03_acnet_templates.tex]

\section{ActivityNet Templates}
\label{appendix:activitynet}

Here we outline the construction process of our silver dataset used for fine-tuning on the \taskname { }task.

\subsection{Data selection}
\label{sub-appendix:activitynet:data-selection}
We select videos from the ActivityNet dataset~\cite{Heilbron_2015_CVPR} because (1) the domain coverage is broad and includes long-form videos with semantically interesting content and (2) multiple follow-up projects have contributed helpful annotations for various related video understanding tasks. Alongside the original ActivityNet dataset labels, we download the annotations produced for the ActivityNet Captions~\cite{Krishna_2017_ICCV} and ActivityNet Entities datasets~\cite{Zhou_2019_CVPR}. ActivityNet Captions provides event segmentation across full ActivityNet videos and fine-grained descriptions of the segmented scenes. ActivityNet Entities builds on ActivityNet Captions, selecting a representative frame from each labeled segment and grounding the relevant nouns mentioned in the captions through spatial bounding boxes.

We download the subset of ActivityNet videos that possess labels from all three datasets and are still available from YouTube.

\subsection{Template selection}
\label{sub-appendix:activitynet:template-selection}
We take the collection of labels from the original ActivityNet annotations applied to our subset of videos, and  organize them into 8 general semantic categories. We then identify a collection of 8 matching FrameNet templates that best approximate the category type. We perform a similar text-to-vision template type conversion done to construct the \dsetname { }ontology, resulting in a collection of vision-centric event templates detailed in Table 7. Each video is mapped to its corresponding template based on semantic category. 

\subsection{Template mapping}
\label{sub-appendix:activitynet:template-mapping}
We pass each ActivityNet Captions description to GPT-4 alongside the question-formatted descriptions of each corresponding event template field. This prompt is included in Appendix A in Figure~\ref{prompt:acnet_templates}. We explain that the description mentions the activity labeled in the original ActivityNet dataset, and ask the model to identify the nouns that could answer the questions. Unlike in our \dsetname {}experiments, we specify that these should be nouns, since only the nouns are grounded in-frame by ActivityNet Entities. We use these GPT-retrieved nouns to assign template field labels to the description text spans, temporal segments as defined by ActivityNet Captions, and the spatial segments as defined by ActivityNet Entities.

\subsection{Silver dataset statistics}
\label{sub-appendix:activitynet:data-stats}
