# Supplementary material for: Grounding Partially-Defined Events in Multimodal Data
Source: arXiv:2410.05267 source file (2024-10-07)
Supplement: Supplementary file 6 [file a11_unused_ontologies.tex]

\begin{table}[t!]
    \small
    \centering
    \caption{ActivityNet Templates ontology, used for silver data fine-tuning. (Part 1/2)}
    \begin{tabular}{p{2.5cm}p{4.5cm}}
    \toprule
        \textbf{Field Name} & \textbf{Field Description}\\
        \midrule
        
        \multicolumn{2}{c}{\textbf{Activity}}\\
    \midrule
         \textbf{Agent} & Who is participating in the activity? \\
         \textbf{Activity} & What activity is being performed? \\
         \textbf{Place} & Where is the activity taking place? \\
         \textbf{Time} & When is the activity taking place? \\
    \midrule

            \multicolumn{2}{c}{\textbf{Building}}\\
    \midrule
         \textbf{Agent} & Who is participating in the activity? \\
         \textbf{Components} & What materials are being used for the project? \\
         \textbf{Created-entity} & What is being built/fixed/crafted? \\
         \textbf{Instrument} & What tool is being used? \\
         \textbf{Place} & Where is the activity taking place? \\
         \textbf{Time} & When is the activity taking place? \\
    \midrule

            \multicolumn{2}{c}{\textbf{Competition}}\\
    \midrule
         \textbf{Competition} & What is the competition? \\
         \textbf{Participants} & Who is participating in the activity? \\
         \textbf{Means} & How are the participants participating in the competition? \\
         \textbf{Place} & Where is the activity taking place? \\
         \textbf{Time} & When is the activity taking place? \\
    \midrule

            \multicolumn{2}{c}{\textbf{Cooking}}\\
    \midrule
         \textbf{Cook} & Who is participating in the activity? \\
         \textbf{Produced-food} & What food is being prepared? \\
         \textbf{Container} & What container is the food being prepared in? \\
         \textbf{Heating-instrument} & What is being used to heat the food? \\
         \textbf{Ingredients} & What ingredients are being used? \\
         \textbf{Recipient} & Who is the recipient of the food? \\
         \textbf{Place} & Where is the activity taking place? \\
         \textbf{Time} & When is the activity taking place? \\
    \midrule

            \multicolumn{2}{c}{\textbf{Exercising}}\\
    \midrule
         \textbf{Agent} & Who is participating in the activity? \\
         \textbf{Body-part} & What part of the body is being exercised? \\
         \textbf{Means} & What are they using to exercise? \\
         \textbf{Place} & Where is the activity taking place? \\
         \textbf{Time} & When is the activity taking place? \\
    \midrule

            \multicolumn{2}{c}{\textbf{Emptying}}\\
    \midrule
         \textbf{Agent} & Who is participating in the activity? \\
         \textbf{Source} & What object/entity is being cleaned/prepared/etc.? \\
         \textbf{Instrument} & What tool is being used by the participant? \\
         \textbf{Result} & What is the result of the activity? \\
         \textbf{Place} & Where is the activity taking place? \\
         \textbf{Time} & When is the activity taking place? \\
        \bottomrule
    \end{tabular}
    \label{tab:acnet-ontology-1}
\end{table}

\begin{table}[t!]
    \small
    \centering
    \caption{ActivityNet Templates ontology, used for silver data fine-tuning. (Part 2/2)}
    \begin{tabular}{p{2.5cm}p{4.5cm}}
    \toprule
        \textbf{Field Name} & \textbf{Field Description}\\
        \midrule
        \multicolumn{2}{c}{\textbf{Grooming}}\\
    \midrule
         \textbf{Agent} & Who is the subject participating in the activity? \\
         \textbf{Patient} & Who is the recipient in the activity (can be the subject themself)? \\
         \textbf{Body-part} & What part of the person is being cared for/groomed? \\
         \textbf{Instrument} & What tool is being used? \\
         \textbf{Result} & What is the result of the care/grooming/activity? \\
         \textbf{Place} & Where is the activity taking place? \\
         \textbf{Time} & When is the activity taking place? \\
    \midrule

            \multicolumn{2}{c}{\textbf{Participation}}\\
    \midrule
         \textbf{Event} & What activity are people participating in? \\
         \textbf{Participants} & Who is participating? \\
         \textbf{Means} & How are the people participating? \\
         \textbf{Place} & Where are people participating? \\
         \textbf{Time} & When are people participating? \\
    \midrule

                \multicolumn{2}{c}{\textbf{Performing Arts}}\\
    \midrule
         \textbf{Audience} & Who is watching the activity? \\
         \textbf{Medium} & What instrument is being used? \\
         \textbf{Performer} & Who is the subject participating in the activity? \\
         \textbf{Personnel} & Who is assisting the main subject participating? \\
         \textbf{Type} & What type of performance is happening? \\
        \bottomrule
    \end{tabular}
    \label{tab:acnet-ontology-2}
\end{table}
